# Supplementary material for: Boosting Online 3D Multi-Object Tracking through Camera-Radar Cross Check
Source: arXiv:2407.13937 source file (2024-07-18)
Supplement: Supplementary file 1 [file n_supplementary.tex]

% \appendix

\setcounter{figure}{0}
\setcounter{table}{0}

% \paragraph{The appendix is structured as follow}
The appendix is structured as follows
\begin{itemize}
    \item We analyze the results of CRAFTBooster from different perspectives, such as related distance, azimuth, and occlusion rate. 
    \item We provide video results from various scenarios, including scenes in different weather conditions.The file is named demo\_CRAFTBooster.mp4.
\end{itemize}
\section{Performance Analysis}

\paragraph{The relative distance} 
between the ego car and surrounding objects plays a pivotal role in influencing the performance, as evidenced by the comprehensive data presented in Table~\ref{tab:Performance_Range}. Recognizing the significance of this factor, our analysis involves categorizing all objects within each specific scenario in K-Radar dataset based on their varying distances from the ego car. This meticulous categorization allows us to delve into a nuanced examination of the TP, FP, and FN values associated with each distance range. The recall metrics further enrich our evaluation, providing a holistic understanding of the system's performance across diverse spatial dimensions. 
As FP increase, precision becomes less stable. This is a problem we mentioned in the limitations section, and addressing this issue is a future goal.

% between the ego car and the object is a crucial influencing factor, as shown in Table~\ref{tab:Performance_Range}. Therefore, we categorize all objects within each scenario in K-Radar based on different distances and analyze the values of TP, FP, and FN. We also observe the differences using precision and recall metrics. In general, as the distance increases, the recall tends to decrease, which aligns with our expectations. Moreover, our method demonstrates the ability to improve the results within any distance range. blank blank blank blank blank blank blank blank blank blank blank blank blank blank blank blank blank blank blank blank blank blank blank blank blank blank blank blank blank blank blank blank blank blank blank blank blank blank blank blank blank blank blank blank blank blank blank blank blank blank blank blank blank blank blank 

\begin{table}[!h]
    \centering
    \resizebox{1\linewidth}{!}{
    \begin{tabular}{cccccccc}
        \toprule
         \makecell[c]{Modality}&\makecell[c]{Relative\\Distance~(m)}& \makecell[c]{Recall$\uparrow$} & \makecell[c]{Precision$\uparrow$\\ }&TP$\uparrow$&FP$\downarrow$&FN$\downarrow$ & \# objs\\
        \midrule
        \multirowcell{8}{BOTSORT\\-Camera}&0-10& 42.7 & 88.5 & 714 & 93 & 958 & 1672  \\ 
        &10-20 & 50.2 & 87.3 & 2,908 & 423   & 2,888 & 5,796 \\ 
        &20-30 & 44.4 & 79.3 & 2,493 & 652   & 3,123 & 5,616 \\
        &30-40 & 42.9 & 68.6 & 2,191 & 1,003 & 2,916 & 5,107 \\
        &40-50 & 38.3 & 57.7 & 1,630 & 1,193 & 2,628 & 4,258 \\
        &50-60 & 37.3 & 53.7 & 1,723 & 1,484 & 2,899 & 4,622 \\
        &60-70 & 22.7 & 40.6 & 741   & 1,084 & 2,527 & 3,268 \\
        &70+   & 8.3  & 28.1 & 52    & 133   & 574   & 626 \\
        \midrule
        \multirowcell{8}{BOTSORT\\-Radar}&0-10& 67.8 & 83.2 & 1133 & 229 & 539 & 1672 \\ 
        &10-20 & 60.0 & 90.3 & 3,480 & 375 & 2,316 & 5,796  \\ 
        &20-30 & 50.0 & 90.8 & 2,807 & 286 & 2,809 & 5,616  \\
        &30-40 & 52.5 & 89.2 & 2,683 & 326 & 2,424 & 5,107  \\
        &40-50 & 52.7 & 87.8 & 2,243 & 313 & 2,015 & 4,258  \\
        &50-60 & 48.6 & 85.4 & 2,245 & 383 & 2,377 & 4,622  \\
        &60-70 & 42.5 & 81.5 & 1,388 & 316 & 1,880 & 3,268  \\
        &70+   & 26.7 & 61.4 & 167   & 105 & 459   & 626  \\
        \midrule
         \multirowcell{8}{CRAFTBooster\\-Camera\\ and Radar}&0-10& 72.4 & 78.1 & 1,210 & 340 & 462 & 1,672\\ 
        &10-20 & 72.6 & 84.2 & 4,207 & 790   & 1,589 & 5,796 \\ 
        &20-30 & 65.7 & 82.7 & 3,692 & 771   & 1,924 & 5,616 \\
        &30-40 & 65.4 & 76.0 & 3,338 & 1,054 & 1,769 & 5,107 \\
        &40-50 & 63.1 & 72.4 & 2,686 & 1,026 & 1,572 & 4,258 \\
        &50-60 & 59.2 & 64.1 & 2,734 & 1,530 & 1,888 & 4,622 \\
        &60-70 & 47.3 & 54.1 & 1,544 & 1,311 & 1,724 & 3,268 \\
        &70+   & 31.3 & 46.6 & 196   & 226   & 430   & 626  \\

        \bottomrule
    \end{tabular}}
    \caption{Performance Comparison of CRAFTBooster with Baselines under various occlusion rate on K-Radar. The online trackers in CRAFTBooster are based on BOTSORT in two modalities.}
    \label{tab:Performance_Range}
\end{table}

\paragraph{The azimuth} with respect to the direction of the ego car is also a key factor. Indeed, the value of the azimuth does not affect performance. Even the results from the camera or radar may not necessarily vary in quality at different angles. Table~\ref{tab:Performance_azi} is mainly intended to show that our method can improve results within each angle range.

\begin{table}[!h]
    \centering
    \resizebox{1\linewidth}{!}{
    \begin{tabular}{cccccccc}
        \toprule
         \makecell[c]{Modality}&\makecell[c]{Azimuth\\(degree)}& \makecell[c]{Recall$\uparrow$} & \makecell[c]{Precision$\uparrow$\\ }&TP$\uparrow$&FP$\downarrow$&FN$\downarrow$ & \# objs\\
        \midrule
        \multirowcell{5}{BOTSORT\\-Camera}
        &0-10   & 37.4 & 65.8 & 6,993   & 3,635 & 11,680& 18,673   \\ 
        &10-20  & 37.3 & 73.5 & 2,490   & 900   & 4,186 & 6,676\\ 
        &20-30  & 55.2 & 70.0 & 1,568   & 671   & 1,271 & 2,839 \\
        &30-40  & 54.5 & 60.3 & 855     & 562   & 714   & 1,569  \\
        &40+    & 45.2 & 64.8 & 546     & 297   & 662   & 1,208   \\

        \midrule
        \multirowcell{5}{BOTSORT\\-Radar}
        &0-10   & 59.9  & 87.5  & 11,179& 1597  & 7,494 & 18,673  \\ 
        &10-20  & 37.1	& 86.0	& 2,478	& 402     & 4,198 & 6,676  \\
        &20-30  & 45.5	& 89.1	& 1,291	& 158  &	1,548&	2,839  \\
        &30-40  & 44.2	& 88.3	& 693	& 92	&876&	1,569    \\
        &40+    & 41.8	& 85.7	& 505	& 84	&703&	1,208    \\

        \midrule
        \multirowcell{5}{CRAFTBooster\\-Camera\\ and Radar}
        &0-10   & 66.9 &	75.1 &	12,501 & 4,153 &	6,172 &	18,673   \\ 
        &10-20  & 52.2 &	76.1 &	3,484 &	1096 &	3,192 &	6,676 \\ 
        &20-30  & 65.8 &	69.2 &	1,869 &	831 &	970 &	2,839  \\
        &30-40  & 65.5 &	63.3 &	1,028 &	595 &	541 &	1569  \\
        &40+    & 60.0 &	66.0 &	725 & 373 &	483 &	1208    \\

        \bottomrule
    \end{tabular}}
    \caption{Performance Comparison of CRAFTBooster with Baselines under various distance range on K-Radar. The online trackers in CRAFTBooster are based on BOTSORT in two modalities.}
    \label{tab:Performance_azi}
\end{table}

\paragraph{The occlusion rate} has a significant impact on the performance from both radar and camera. We calculate the occlusion rate of all ground truth objects in the image, using the same method as described in \textbf{Cross-modality Check on Unmatched Detections}. Since only ground truth can be used to calculate the occlusion rate, we focus on calculating the recall score. However, our method still effectively improves performance.

\begin{table}[!h]
    \centering
    \resizebox{1\linewidth}{!}{
    \begin{tabular}{cccccc}
        \toprule
         \makecell[c]{Modality}&\makecell[c]{Occlusion Rate}& \makecell[c]{Recall$\uparrow$} & TP$\uparrow$ &FN$\downarrow$ & \# objs\\
        \midrule
        \multirowcell{4}{BOTSORT\\-Camera}
        &0.00-0.25  &41.9   & 10,353 & 14,363 & 24,716 \\ 
        &0.25-0.50  & 37.4  & 866   & 1,451  & 2,317  \\ 
        &0.50-0.75  & 32.1  & 717   & 1,517  & 2,234 \\
        &0.75-1.00  & 30.4  & 516   & 1,182  & 1,698 \\
        \midrule
        \multirowcell{4}{BOTSORT\\-Radar}
        &0.00-0.25  & 56.7 & 14,008 & 10,708    & 24,716 \\ 
        &0.25-0.50  & 37.2 & 862    & 1,455     & 2,317  \\ 
        &0.50-0.75  & 28.3 & 633    & 1,601     & 2,234  \\
        &0.75-1.00  & 37.9 & 643    & 1,055     & 1,698  \\
        \midrule
        \multirowcell{4}{CRAFTBooster\\-Camera\\ and Radar}
        &0.00-0.25  & 67.0 & 16,547 & 8,169 & 24,716      \\ 
        &0.25-0.50  & 52.8 & 1,223  & 1,094 & 2,317   \\ 
        &0.50-0.75  & 42.6 & 951    & 1283  & 2,234   \\
        &0.75-1.00  & 52.2 & 886    & 812   & 1,698   \\
        \bottomrule
    \end{tabular}}
    \caption{Performance Comparison of CRAFTBooster with Baselines under various occlusion rate on K-Radar. The online trackers in CRAFTBooster are based on BOTSORT in two modalities.}
    \label{tab:Performance_occ}
\end{table}
